# Supplementary material for: Adaptive Shortcut Debiasing for Online Continual Learning
Source: arXiv:2312.08677 source file (2023-12-14)
Supplement: Supplementary file 1 [file ablation.tex]

% \newcolumntype{C}[1]{>{\centering\arraybackslash}p{#1}}
% \bgroup
% make the row margin compact
\begin{table}[t]
% \small
\scriptsize
% \small
% \label{tbl:RegionBuzComparison}
\centering
\caption{Ablation study on multi-level feature fusion and drop intensity shifting with respect to $A_{avg}$ on Split CIFAR-100. The highest values are marked in bold. }
\vspace*{-0.3cm}
\begin{tabular}[c]
% {@{}c|c|C{1.3cm}C{1.3cm}C{1.3cm}C{1.3cm}C{1.3cm}C{1.3cm}C{1.3cm}C{1.7cm}@{}}
% {@{}c|c||C{0.9cm}C{1.1cm}||C{0.9cm}c@{}}
% {@{}c||C{1.1cm}|C{1.2cm}|C{1.2cm}|C{1.1cm}c@{}}
{@{}l||c|c|c|cc@{}}
\toprule
% \multicolumn{1}{c||}{} & \multicolumn{3}{c|}{\textbf{{    Variants   }}} & \multicolumn{1}{c}{} \\\cline{2-4}
\multicolumn{1}{c||}{\textbf{}} & \multicolumn{1}{c|}{\textbf{}} & \multicolumn{2}{c|}{\textbf{No Drop Int. Shift}} & \multicolumn{1}{c}{} \\
% \smallskip
\multicolumn{1}{c||}{\hspace{-0.3cm}\textbf{Method}} %\textbf{Method}}
& \multicolumn{1}{c|}{\textbf{No MF}\hspace{-1cm}}
& \multicolumn{1}{c|}{\textbf{Rand Drop}}
& \multicolumn{1}{c|}{\textbf{Top Drop}}
& \multicolumn{1}{c}{\textbf{SDOCL}}
% & \multicolumn{1}{c}{\bm{$F_{last}$}}
% & \multicolumn{1}{c|}{\bm{$A_{avg}$}}
% & \multicolumn{1}{c}{\bm{$F_{last}$}}
% & \multicolumn{1}{c|}{\bm{$A_{avg}$}}
% & \multicolumn{1}{c}{\bm{$F_{last}$}}
% & \multicolumn{1}{c}{\bm{$A_{avg}$}}

\\ \toprule
% seq-cifar100---gss---adl_qty_spatialrdl_greedygreedy_10_0.05_0.9_init_0.1_0.0_evalperiod3---drop_thrh0.95_select_drop_prob1.0_gating_pos4_mean_accs_classil.csv
% & \begin{tabular}[c]{@{}c@{}}{ {19.98}\,($\pm$0.14) }\end{tabular}
% & \begin{tabular}[c]{@{}c@{}}{ {22.22}\,($\pm$0.53) }\end{tabular}

% seq-cifar100---mir---adl_qty_spatialrdl_greedygreedy_10_0.05_0.9_evalperiod3---drop_thrh0.95_select_drop_prob1.0_gating_pos4_mean_accs_classil.csv
% & \begin{tabular}[c]{@{}c@{}}{ {21.9}\,($\pm$0.24) }\end{tabular}
% & \begin{tabular}[c]{@{}c@{}}{ {27.4}\,($\pm$0.74) }\end{tabular}

% seq-cifar100---aser---adl_qty_spatialrdl_greedygreedy_10_0.05_0.9_init_0.1_0.0_evalperiod3---drop_thrh0.95_select_drop_prob1.0_gating_pos4_mean_accs_classil.csv
% & \begin{tabular}[c]{@{}c@{}}{ {30.62}\,($\pm$0.31) }\end{tabular}
% & \begin{tabular}[c]{@{}c@{}}{ {37.82}\,($\pm$0.55) }\end{tabular}

% seq-cifar100---er---adl_qty_spatialrdl_greedygreedy_10_0.05_0.9_evalperiod3---drop_thrh0.95_select_drop_prob1.0_gating_pos4_mean_accs_classil.csv
% & \begin{tabular}[c]{@{}c@{}}{ {26.17}\,($\pm$0.15) }\end{tabular}
% & \begin{tabular}[c]{@{}c@{}}{ {18.82}\,($\pm$0.18) }\end{tabular}

% seq-cifar100---derpp---adl_qty_spatialrdl_greedygreedy_10_0.05_0.9_evalperiod3---drop_thrh0.95_select_drop_prob1.0_gating_pos4_mean_accs_classil.csv
% & \begin{tabular}[c]{@{}c@{}}{ {23.36}\,($\pm$0.27) }\end{tabular}
% & \begin{tabular}[c]{@{}c@{}}{ {29.13}\,($\pm$0.39) }\end{tabular}
% # ER ###############################################################
\multirow{1}{*}{ER~\cite{rolnick2019experience}\hspace{-0.15cm}}                                
& \begin{tabular}[c]{@{}c@{}}{{26.2}\,($\pm$0.2)\hspace{-1cm}}\end{tabular}
& \begin{tabular}[c]{@{}c@{}}{{25.5}\,($\pm$0.3)}\end{tabular}
& \begin{tabular}[c]{@{}c@{}}{{25.5}\,($\pm$0.2)}\end{tabular}
& \begin{tabular}[c]{@{}c@{}}{\textbf{{ 26.5 }}\,($\pm$0.2)}\end{tabular}
\\
% \midrule
% \cdashline{}
% # ER ###############################################################

% DER ++ ###############################################################
\multirow{1}{*}{DER++~\cite{buzzega2020dark}\hspace{-0.15cm}}                                                   
& \begin{tabular}[c]{@{}c@{}}{{23.4}\,($\pm$0.3)\hspace{-1cm}}\end{tabular}
& \begin{tabular}[c]{@{}c@{}}{{22.0}\,($\pm$0.2)}\end{tabular}
& \begin{tabular}[c]{@{}c@{}}{{24.2}\,($\pm$0.3)}\end{tabular}
& \begin{tabular}[c]{@{}c@{}}{\textbf{{ 25.1 }}\,($\pm$0.3)}\end{tabular}
\\
% \midrule
% % # ++ ###############################################################

% # MIR ################################################################
\multirow{1}{*}{MIR~\cite{mir}\hspace{-0.15cm}}                                               
& \begin{tabular}[c]{@{}c@{}}{{21.9}\,($\pm$0.2)\hspace{-1cm}}\end{tabular}
& \begin{tabular}[c]{@{}c@{}}{{22.5}\,($\pm$0.7)}\end{tabular}
& \begin{tabular}[c]{@{}c@{}}{{22.4}\,($\pm$0.3)}\end{tabular}
& \begin{tabular}[c]{@{}c@{}}{{22.4}\,($\pm$0.1)}\end{tabular}
\\

% # GSS ################################################################
\multirow{1}{*}{GSS~\cite{aljundi2019gradient}\hspace{-0.15cm}}                                 
& \begin{tabular}[c]{@{}c@{}}{{20.0}\,($\pm$0.1)\hspace{-1cm}}\end{tabular}
& \begin{tabular}[c]{@{}c@{}}{{20.7}\,($\pm$0.2)}\end{tabular}
& \begin{tabular}[c]{@{}c@{}}{{22.7}\,($\pm$0.3)}\end{tabular}
& \begin{tabular}[c]{@{}c@{}}{\textbf{{23.7}}\,($\pm$0.2)}\end{tabular}
\\
% \midrule

% # ASER ################################################################
\multirow{1}{*}{ASER~\cite{shim2021online}\hspace{-0.15cm}}                                               
& \begin{tabular}[c]{@{}c@{}}{{30.6}\,($\pm$0.3)\hspace{-1cm}}\end{tabular}
& \begin{tabular}[c]{@{}c@{}}{\textbf{{34.2}}\,($\pm$0.1)}\end{tabular}
& \begin{tabular}[c]{@{}c@{}}{{31.8}\,($\pm$0.2)}\end{tabular}
& \begin{tabular}[c]{@{}c@{}}{{33.4}\,($\pm$0.4)}\end{tabular}
\\
\midrule
% \cdashline{}

\multirow{1}{*}{\textbf{AVG}\,\textbf{(Degrad.)}\hspace{-0.15cm}}                                               
% # AVG ################################################################
& \begin{tabular}[c]{@{}c@{}}{{24.4}\,(\textbf{-7.4\%})\hspace{-1cm}}\end{tabular}
& \begin{tabular}[c]{@{}c@{}}{{25.0}\,(\textbf{-4.8\%})}\end{tabular}
& \begin{tabular}[c]{@{}c@{}}{{25.3}\,(\textbf{-3.6\%})}\end{tabular}
& \begin{tabular}[c]{@{}c@{}}{\textbf{{26.2}}}\end{tabular}
% \\
% \multirow{1}{*}{\textbf{Degrad}}                                               
% & \begin{tabular}[c]{@{}c@{}}{ {24.4} }\end{tabular}
% & \begin{tabular}[c]{@{}c@{}}{ {25.3} }\end{tabular}
% & \begin{tabular}[c]{@{}c@{}}{ {25.0} }\end{tabular}
% & \begin{tabular}[c]{@{}c@{}}{ \textbf{{26.2}} }\end{tabular}
\\
\bottomrule
\end{tabular}
\label{tbl:ablation}

\end{table}
