# Supplementary material for: Adaptive Shortcut Debiasing for Online Continual Learning
Source: arXiv:2312.08677 source file (2023-12-14)
Supplement: Supplementary file 3 [file overall_performance.tex]

% \newcolumntype{C}[1]{>{\centering\arraybackslash}p{#1}}
% \bgroup
% make the row margin compact
\begin{table*}[t]
% \small
\scriptsize
% \small
% \label{tbl:RegionBuzComparison}
\centering
\caption{Performance comparisons on CIFAR10, CIFAR100, and SuperImageNet-9 for biased setup. The highest values are marked in bold. The mean of \emph{five} repetitions with different random initialization were reported. }
\begin{tabular}[c]
% {@{}c|c|C{1.3cm}C{1.3cm}C{1.3cm}C{1.3cm}C{1.3cm}C{1.3cm}C{1.3cm}C{1.7cm}@{}}
{@{}c|c||cc|cc|cc|cc|ccc@{}}
% {@{}c|c|ccccccccc@{}}
\toprule
\multicolumn{1}{c|}{} & \multicolumn{1}{c||}{} & \multicolumn{6}{c|}{\textbf{\underline{    Biased Setup    }}} & \multicolumn{4}{c}{\textbf{\underline{    Unbiased Setup   }}} \\
\multicolumn{1}{c|}{} & \multicolumn{1}{c||}{} & \multicolumn{2}{c}{\textbf{CIFAR10}} & \multicolumn{2}{c}{\textbf{CIFAR100}} & \multicolumn{2}{c|}{\textbf{IN-9}} & \multicolumn{2}{c}{\textbf{IN-OnlyFG}} & \multicolumn{2}{c}{\textbf{IN-Stylized}} \\
% \smallskip
\multicolumn{1}{c|}{\textbf{Method}}
& \multicolumn{1}{c||}{\textbf{Debias Method}}
& \multicolumn{1}{c}{\bm{$F_{last}$}}
& \multicolumn{1}{c|}{\bm{$A_{avg}$}}
& \multicolumn{1}{c}{\bm{$F_{last}$}}
& \multicolumn{1}{c|}{\bm{$A_{avg}$}}
& \multicolumn{1}{c}{\bm{$F_{last}$}}
& \multicolumn{1}{c|}{\bm{$A_{avg}$}}
& \multicolumn{1}{c}{\bm{$F_{last}$}}
& \multicolumn{1}{c|}{\bm{$A_{avg}$}}
& \multicolumn{1}{c}{\bm{$F_{last}$}}
& \multicolumn{1}{c}{\bm{$A_{avg}$}}

\\ \toprule
% # ER ###############################################################
\multirow{2}{*}{ER}                                
& \begin{tabular}[c]{@{}c@{}}\textrm{ -- }\end{tabular}
& \begin{tabular}[c]{@{}c@{}}{ { 39.89 }\,($\pm$2.35) }\end{tabular}
& \begin{tabular}[c]{@{}c@{}}{ { 55.36 }\,($\pm$0.30) }\end{tabular}
& \begin{tabular}[c]{@{}c@{}}{ { 19.22 }\,($\pm$0.25) }\end{tabular}
& \begin{tabular}[c]{@{}c@{}}{ { 25.34 }\,($\pm$0.18) }\end{tabular}
& \begin{tabular}[c]{@{}c@{}}{ {50.95}\,($\pm$2.14) }\end{tabular}
& \begin{tabular}[c]{@{}c@{}}{ {44.48}\,($\pm$1.38) }\end{tabular}

& \begin{tabular}[c]{@{}c@{}}{ 17.6 }\end{tabular}
& \begin{tabular}[c]{@{}c@{}}{ 28.9 }\end{tabular}
& \begin{tabular}[c]{@{}c@{}}{ 29.1 }\end{tabular}
& \begin{tabular}[c]{@{}c@{}}{ \textbf{40.3} }\end{tabular}
\\
& \begin{tabular}[c]{@{}c@{}}\textrm{ SDOCL }\end{tabular}
& \begin{tabular}[c]{@{}c@{}}{ { 37.60 }\,($\pm$1.89) }\end{tabular}
& \begin{tabular}[c]{@{}c@{}}{ { 61.02 }\,($\pm$0.61) }\end{tabular}
& \begin{tabular}[c]{@{}c@{}}{ { 18.28 }\,($\pm$1.31) }\end{tabular}
& \begin{tabular}[c]{@{}c@{}}{ { 26.45 }\,($\pm$0.17) }\end{tabular}
& \begin{tabular}[c]{@{}c@{}}{ {36.12}\,($\pm$4.74) }\end{tabular}
& \begin{tabular}[c]{@{}c@{}}{ {48.94}\,($\pm$1.01) }\end{tabular}

& \begin{tabular}[c]{@{}c@{}}{ \textbf{19.2} ($\pm$ 0.12) }\end{tabular}
& \begin{tabular}[c]{@{}c@{}}{ 28.7 }\end{tabular}
& \begin{tabular}[c]{@{}c@{}}{ \textbf{29.8} }\end{tabular}
& \begin{tabular}[c]{@{}c@{}}{ 39.4 }\end{tabular}
% \\
% & \begin{tabular}[c]{@{}c@{}}\textrm{ Random }\end{tabular}
% & \begin{tabular}[c]{@{}c@{}}{ \textbf{50.6} }\end{tabular}
% & \begin{tabular}[c]{@{}c@{}}{ \textbf{59.9} }\end{tabular}
% & \begin{tabular}[c]{@{}c@{}}{ \textbf{23.8} }\end{tabular}
% & \begin{tabular}[c]{@{}c@{}}{ \textbf{24.1} }\end{tabular}
% & \begin{tabular}[c]{@{}c@{}}{ 32.4 }\end{tabular}
% & \begin{tabular}[c]{@{}c@{}}{ \textbf{45.4} }\end{tabular}
% & \begin{tabular}[c]{@{}c@{}}{ 15.0 }\end{tabular}
% & \begin{tabular}[c]{@{}c@{}}{ \textbf{30.7} }\end{tabular}
% & \begin{tabular}[c]{@{}c@{}}{ 26.7 }\end{tabular}
% & \begin{tabular}[c]{@{}c@{}}{ 39.5 }\end{tabular}
\\
\midrule
% # ER ###############################################################

% DER ++ ###############################################################
\multirow{2}{*}{DER++}                                                         
& \begin{tabular}[c]{@{}c@{}}\textrm{ -- }\end{tabular}
& \begin{tabular}[c]{@{}c@{}}{ { 28.20 }\,($\pm$1.48) }\end{tabular}
& \begin{tabular}[c]{@{}c@{}}{ { 59.76 }\,($\pm$0.76) }\end{tabular}
& \begin{tabular}[c]{@{}c@{}}{ { 33.43 }\,($\pm$0.73) }\end{tabular}
& \begin{tabular}[c]{@{}c@{}}{ { 23.64 }\,($\pm$0.32) }\end{tabular}
& \begin{tabular}[c]{@{}c@{}}{ {63.0}\,($\pm$4.62) }\end{tabular}
& \begin{tabular}[c]{@{}c@{}}{ {44.2}\,($\pm$1.01) }\end{tabular}

& \begin{tabular}[c]{@{}c@{}}{ 12.3 }\end{tabular}
& \begin{tabular}[c]{@{}c@{}}{ 28.2 }\end{tabular}
& \begin{tabular}[c]{@{}c@{}}{ 22.7 }\end{tabular}
& \begin{tabular}[c]{@{}c@{}}{ 37.9 }\end{tabular}
\\
& \begin{tabular}[c]{@{}c@{}}\textrm{ SDOCL }\end{tabular}
& \begin{tabular}[c]{@{}c@{}}{ { 23.68 }\,($\pm$0.98) }\end{tabular}
& \begin{tabular}[c]{@{}c@{}}{ { 62.56 }\,($\pm$0.73) }\end{tabular}
& \begin{tabular}[c]{@{}c@{}}{ { 31.11 }\,($\pm$1.15) }\end{tabular}
& \begin{tabular}[c]{@{}c@{}}{ { 25.14 }\,($\pm$0.27) }\end{tabular}
& \begin{tabular}[c]{@{}c@{}}{ {60.73}\,($\pm$5.06) }\end{tabular}
& \begin{tabular}[c]{@{}c@{}}{ {45.42}\,($\pm$0.54) }\end{tabular}

& \begin{tabular}[c]{@{}c@{}}{ \textbf{13.8} }\end{tabular}
& \begin{tabular}[c]{@{}c@{}}{ \textbf{29.5} }\end{tabular}
& \begin{tabular}[c]{@{}c@{}}{ \textbf{23.5} }\end{tabular}
& \begin{tabular}[c]{@{}c@{}}{ \textbf{38.9} }\end{tabular}
% \\
% & \begin{tabular}[c]{@{}c@{}}\textrm{ Random }\end{tabular}
% & \begin{tabular}[c]{@{}c@{}}{ \textbf{51.1} }\end{tabular}
% & \begin{tabular}[c]{@{}c@{}}{ \textbf{61.1} }\end{tabular}
% & \begin{tabular}[c]{@{}c@{}}{ \textbf{21.1} }\end{tabular}
% & \begin{tabular}[c]{@{}c@{}}{ 23.2 }\end{tabular}
% & \begin{tabular}[c]{@{}c@{}}{ \textbf{30.6 }}\end{tabular}
% & \begin{tabular}[c]{@{}c@{}}{ \textbf{43.5} }\end{tabular}
% & \begin{tabular}[c]{@{}c@{}}{ \textbf{19.6} }\end{tabular}
% & \begin{tabular}[c]{@{}c@{}}{ \textbf{29.0} }\end{tabular}
% & \begin{tabular}[c]{@{}c@{}}{ \textbf{26.7} }\end{tabular}
% & \begin{tabular}[c]{@{}c@{}}{ \textbf{38.5} }\end{tabular}
\\
\midrule
% % # ++ ###############################################################

% # MIR ################################################################
\multirow{2}{*}{MIR}                                               
& \begin{tabular}[c]{@{}c@{}}\textrm{ -- }\end{tabular}
& \begin{tabular}[c]{@{}c@{}}{ {58.42}\,($\pm$1.28) }\end{tabular}
& \begin{tabular}[c]{@{}c@{}}{ {51.54}\,($\pm$0.5) }\end{tabular}
& \begin{tabular}[c]{@{}c@{}}{ {25.32}\,($\pm$1.69) }\end{tabular}
& \begin{tabular}[c]{@{}c@{}}{ {20.75}\,($\pm$0.56) }\end{tabular}
& \begin{tabular}[c]{@{}c@{}}{ {41.07}\,($\pm$1.99) }\end{tabular}
& \begin{tabular}[c]{@{}c@{}}{ {39.34}\,($\pm$1.18) }\end{tabular}

& \begin{tabular}[c]{@{}c@{}}{ 16.9 }\end{tabular}
& \begin{tabular}[c]{@{}c@{}}{ 28.9 }\end{tabular}
& \begin{tabular}[c]{@{}c@{}}{ 37.3 }\end{tabular}
& \begin{tabular}[c]{@{}c@{}}{ 46.1 }\end{tabular}
\\
& \begin{tabular}[c]{@{}c@{}}\textrm{ SDOCL }\end{tabular}
& \begin{tabular}[c]{@{}c@{}}{ {56.25}\,($\pm$1.58) }\end{tabular}
& \begin{tabular}[c]{@{}c@{}}{ {51.63}\,($\pm$0.56) }\end{tabular}
& \begin{tabular}[c]{@{}c@{}}{ {25.06}\,($\pm$1.05) }\end{tabular}
& \begin{tabular}[c]{@{}c@{}}{ {21.72}\,($\pm$0.34) }\end{tabular}
& \begin{tabular}[c]{@{}c@{}}{ {39.25}\,($\pm$4.47) }\end{tabular}
& \begin{tabular}[c]{@{}c@{}}{ {42.01}\,($\pm$0.93) }\end{tabular}

& \begin{tabular}[c]{@{}c@{}}{ \textbf{18.9} }\end{tabular}
& \begin{tabular}[c]{@{}c@{}}{ \textbf{36.5} }\end{tabular}
& \begin{tabular}[c]{@{}c@{}}{ \textbf{39.4}}\end{tabular}
& \begin{tabular}[c]{@{}c@{}}{ \textbf{50.7} }\end{tabular}
% \\
% & \begin{tabular}[c]{@{}c@{}}\textrm{ Random }\end{tabular}
% & \begin{tabular}[c]{@{}c@{}}{ \textbf{62.7} }\end{tabular}
% & \begin{tabular}[c]{@{}c@{}}{ \textbf{69.5} }\end{tabular}
% & \begin{tabular}[c]{@{}c@{}}{ 35.0 }\end{tabular}
% & \begin{tabular}[c]{@{}c@{}}{ \textbf{31.1} }\end{tabular}
% & \begin{tabular}[c]{@{}c@{}}{ \textbf{52.4} }\end{tabular}
% & \begin{tabular}[c]{@{}c@{}}{ \textbf{56.5} }\end{tabular}
% & \begin{tabular}[c]{@{}c@{}}{ \textbf{20.0} }\end{tabular}
% & \begin{tabular}[c]{@{}c@{}}{ \textbf{33.6} }\end{tabular}
% & \begin{tabular}[c]{@{}c@{}}{\textbf{39.8} }\end{tabular}
% & \begin{tabular}[c]{@{}c@{}}{ \textbf{50.6} }\end{tabular}
\\
\midrule

% # GSS ################################################################
\multirow{2}{*}{GSS}                                               
& \begin{tabular}[c]{@{}c@{}}\textrm{ -- }\end{tabular}
& \begin{tabular}[c]{@{}c@{}}{ {69.66}\,($\pm$0.71) }\end{tabular}
& \begin{tabular}[c]{@{}c@{}}{ {46.04}\,($\pm$0.42) }\end{tabular}
& \begin{tabular}[c]{@{}c@{}}{ {24.22}\,($\pm$0.73) }\end{tabular}
& \begin{tabular}[c]{@{}c@{}}{ {20.95}\,($\pm$0.37) }\end{tabular}
& \begin{tabular}[c]{@{}c@{}}{ {71.53}\,($\pm$2.01) }\end{tabular}
& \begin{tabular}[c]{@{}c@{}}{ {40.33}\,($\pm$0.63) }\end{tabular}

& \begin{tabular}[c]{@{}c@{}}{ 16.9 }\end{tabular}
& \begin{tabular}[c]{@{}c@{}}{ 28.9 }\end{tabular}
& \begin{tabular}[c]{@{}c@{}}{ 37.3 }\end{tabular}
& \begin{tabular}[c]{@{}c@{}}{ 46.1 }\end{tabular}
\\
& \begin{tabular}[c]{@{}c@{}}\textrm{ SDOCL }\end{tabular}
& \begin{tabular}[c]{@{}c@{}}{ {69.22}\,($\pm$1.53) }\end{tabular}
& \begin{tabular}[c]{@{}c@{}}{ {49.05}\,($\pm$0.46) }\end{tabular}
& \begin{tabular}[c]{@{}c@{}}{ {29.06}\,($\pm$0.87) }\end{tabular}
& \begin{tabular}[c]{@{}c@{}}{ {24.45}\,($\pm$0.27) }\end{tabular}
& \begin{tabular}[c]{@{}c@{}}{ {68.53}\,($\pm$1.87) }\end{tabular}
& \begin{tabular}[c]{@{}c@{}}{ {41.26}\,($\pm$0.57) }\end{tabular}

& \begin{tabular}[c]{@{}c@{}}{ \textbf{18.9} }\end{tabular}
& \begin{tabular}[c]{@{}c@{}}{ \textbf{36.5} }\end{tabular}
& \begin{tabular}[c]{@{}c@{}}{ \textbf{39.4}}\end{tabular}
& \begin{tabular}[c]{@{}c@{}}{ \textbf{50.7} }\end{tabular}
% \\
% & \begin{tabular}[c]{@{}c@{}}\textrm{ Random }\end{tabular}
% & \begin{tabular}[c]{@{}c@{}}{ \textbf{62.7} }\end{tabular}
% & \begin{tabular}[c]{@{}c@{}}{ \textbf{69.5} }\end{tabular}
% & \begin{tabular}[c]{@{}c@{}}{ 35.0 }\end{tabular}
% & \begin{tabular}[c]{@{}c@{}}{ \textbf{31.1} }\end{tabular}
% & \begin{tabular}[c]{@{}c@{}}{ \textbf{52.4} }\end{tabular}
% & \begin{tabular}[c]{@{}c@{}}{ \textbf{56.5} }\end{tabular}
% & \begin{tabular}[c]{@{}c@{}}{ \textbf{20.0} }\end{tabular}
% & \begin{tabular}[c]{@{}c@{}}{ \textbf{33.6} }\end{tabular}
% & \begin{tabular}[c]{@{}c@{}}{\textbf{39.8} }\end{tabular}
% & \begin{tabular}[c]{@{}c@{}}{ \textbf{50.6} }\end{tabular}
\\
\midrule

% # ASER ################################################################
\multirow{2}{*}{ASER}                                               
& \begin{tabular}[c]{@{}c@{}}\textrm{ -- }\end{tabular}
& \begin{tabular}[c]{@{}c@{}}{ { 57.77 }\,($\pm$3.33) }\end{tabular}
& \begin{tabular}[c]{@{}c@{}}{ { 50.32 }\,($\pm$0.45) }\end{tabular}
& \begin{tabular}[c]{@{}c@{}}{ { 41.77 }\,($\pm$0.41) }\end{tabular}
& \begin{tabular}[c]{@{}c@{}}{ { 32.68 }\,($\pm$0.10) }\end{tabular}
& \begin{tabular}[c]{@{}c@{}}{ {62.63}\,($\pm$2.05) }\end{tabular}
& \begin{tabular}[c]{@{}c@{}}{ {39.7}\,($\pm$0.72) }\end{tabular}

& \begin{tabular}[c]{@{}c@{}}{ 16.9 }\end{tabular}
& \begin{tabular}[c]{@{}c@{}}{ 28.9 }\end{tabular}
& \begin{tabular}[c]{@{}c@{}}{ 37.3 }\end{tabular}
& \begin{tabular}[c]{@{}c@{}}{ 46.1 }\end{tabular}
\\
& \begin{tabular}[c]{@{}c@{}}\textrm{ SDOCL }\end{tabular}
& \begin{tabular}[c]{@{}c@{}}{ { 57.54 }\,($\pm$0.75) }\end{tabular}
& \begin{tabular}[c]{@{}c@{}}{ { 51.32 }\,($\pm$0.32) }\end{tabular}
& \begin{tabular}[c]{@{}c@{}}{ { 39.54 }\,($\pm$0.81) }\end{tabular}
& \begin{tabular}[c]{@{}c@{}}{ { 33.43 }\,($\pm$0.38) }\end{tabular}
& \begin{tabular}[c]{@{}c@{}}{ {57.5}\,($\pm$3.18) }\end{tabular}
& \begin{tabular}[c]{@{}c@{}}{ {41.6}\,($\pm$0.76) }\end{tabular}

& \begin{tabular}[c]{@{}c@{}}{ \textbf{18.9} }\end{tabular}
& \begin{tabular}[c]{@{}c@{}}{ \textbf{36.5} }\end{tabular}
& \begin{tabular}[c]{@{}c@{}}{ \textbf{39.4}}\end{tabular}
& \begin{tabular}[c]{@{}c@{}}{ \textbf{50.7} }\end{tabular}
% \\
% & \begin{tabular}[c]{@{}c@{}}\textrm{ Random }\end{tabular}
% & \begin{tabular}[c]{@{}c@{}}{ \textbf{62.7} }\end{tabular}
% & \begin{tabular}[c]{@{}c@{}}{ \textbf{69.5} }\end{tabular}
% & \begin{tabular}[c]{@{}c@{}}{ 35.0 }\end{tabular}
% & \begin{tabular}[c]{@{}c@{}}{ \textbf{31.1} }\end{tabular}
% & \begin{tabular}[c]{@{}c@{}}{ \textbf{52.4} }\end{tabular}
% & \begin{tabular}[c]{@{}c@{}}{ \textbf{56.5} }\end{tabular}
% & \begin{tabular}[c]{@{}c@{}}{ \textbf{20.0} }\end{tabular}
% & \begin{tabular}[c]{@{}c@{}}{ \textbf{33.6} }\end{tabular}
% & \begin{tabular}[c]{@{}c@{}}{\textbf{39.8} }\end{tabular}
% & \begin{tabular}[c]{@{}c@{}}{ \textbf{50.6} }\end{tabular}
\\
\bottomrule

\end{tabular}
\label{tbl:overall_comparison_biased_setup}
\end{table*}
