# Supplementary material for: Adaptive Shortcut Debiasing for Online Continual Learning
Source: arXiv:2312.08677 source file (2023-12-14)
Supplement: Supplementary file 4 [file performance_biased_setup.tex]

\newcolumntype{C}[1]{>{\centering\arraybackslash}p{#1}}
% \bgroup
% make the row margin compact
\begin{table*}[t]
\small
\scriptsize
% \small
% \label{tbl:RegionBuzComparison}
\centering
\caption{Average accuracy\,(higher is better) and forgetting\,(lower is better) on Split CIFAR-100, Split CIFAR-10, and Split ImageNet-9 for biased setup\,(The best results are marked in bold). The mean of \emph{five} repetitions with different random initialization were reported. }
\resizebox{1.0\linewidth}{!}{%
\begin{tabular}[c]
% {@{}c|c|C{1.3cm}C{1.3cm}C{1.3cm}C{1.3cm}C{1.3cm}C{1.3cm}C{1.3cm}C{1.7cm}@{}}
{@{}l|c||C{1.85cm}c|C{1.85cm}c|C{1.85cm}cc@{}}
% {@{}c|c|ccccccccc@{}}
\toprule
\multicolumn{1}{c|}{} & \multicolumn{1}{c||}{} & \multicolumn{6}{c}{\textbf{\underline{    Biased Setup    }}} \\
% & \multicolumn{4}{c}{\textbf{{    Unbiased Setup   }}} \\
\multicolumn{1}{c|}{\textbf{OCL}} & \multicolumn{1}{c||}{\textbf{Debias}} & \multicolumn{2}{c}{\textbf{Split CIFAR-100}} & \multicolumn{2}{c}{\textbf{Split CIFAR-10}} & \multicolumn{2}{c}{\textbf{Split ImageNet-9}} \\
% & \multicolumn{2}{c}{\textbf{IN-OnlyFG}} & \multicolumn{2}{c}{\textbf{IN-Stylized}} \\
% \smallskip
\multicolumn{1}{c|}{\textbf{Method}}
& \multicolumn{1}{c||}{\textbf{Method}}
& \multicolumn{1}{c}{\bm{$A_{avg}$}\,($\uparrow$)}
& \multicolumn{1}{c|}{\bm{$F_{last}$}\,($\downarrow$)}
& \multicolumn{1}{c}{\bm{$A_{avg}$}\,($\uparrow$)}
& \multicolumn{1}{c|}{\bm{$F_{last}$}\,($\downarrow$)}
& \multicolumn{1}{c}{\bm{$A_{avg}$}\,($\uparrow$)}
& \multicolumn{1}{c}{\bm{$F_{last}$}\,($\downarrow$)}
% & \multicolumn{1}{c}{\bm{$A_{avg}$}}
% & \multicolumn{1}{c|}{\bm{$F_{last}$}}
% & \multicolumn{1}{c}{\bm{$A_{avg}$}}
% & \multicolumn{1}{c}{\bm{$F_{last}$}}
\\ \toprule
% # ER ###############################################################
\multirow{2}{*}{ER~\cite{rolnick2019experience}}                                
& \begin{tabular}[c]{@{}c@{}}\textrm{ -- }\end{tabular}
& \begin{tabular}[c]{@{}c@{}}{ {25.34}\,($\pm$0.18) }\end{tabular}
& \begin{tabular}[c]{@{}c@{}}{ {19.22}\,($\pm$0.25) }\end{tabular}
& \begin{tabular}[c]{@{}c@{}}{ {55.36}\,($\pm$0.30) }\end{tabular}
& \begin{tabular}[c]{@{}c@{}}{ {39.89}\,($\pm$2.35) }\end{tabular}
& \begin{tabular}[c]{@{}c@{}}{ {46.05}\,($\pm$0.20) }\end{tabular}
& \begin{tabular}[c]{@{}c@{}}{ {55.80}\,($\pm$1.82) }\end{tabular}
% & \begin{tabular}[c]{@{}c@{}}{ 17.6 }\end{tabular}
% & \begin{tabular}[c]{@{}c@{}}{ 28.9 }\end{tabular}
% & \begin{tabular}[c]{@{}c@{}}{ 29.1 }\end{tabular}
% & \begin{tabular}[c]{@{}c@{}}{ \textbf{40.3} }\end{tabular}
\\
& \begin{tabular}[c]{@{}c@{}}\textrm{ SDOCL }\end{tabular}
& \begin{tabular}[c]{@{}c@{}}{ \textbf{26.45}\,($\pm$0.17) }\end{tabular}
& \begin{tabular}[c]{@{}c@{}}{ \textbf{18.28}\,($\pm$1.31) }\end{tabular}
& \begin{tabular}[c]{@{}c@{}}{ \textbf{61.02}\,($\pm$0.61) }\end{tabular}
& \begin{tabular}[c]{@{}c@{}}{ \textbf{37.60}\,($\pm$1.89) }\end{tabular}
& \begin{tabular}[c]{@{}c@{}}{ \textbf{48.86}\,($\pm$0.43) }\end{tabular}
& \begin{tabular}[c]{@{}c@{}}{ \textbf{44.01}\,($\pm$3.76) }\end{tabular}
% & \begin{tabular}[c]{@{}c@{}}{ \textbf{19.2} ($\pm$ 0.12) }\end{tabular}
% & \begin{tabular}[c]{@{}c@{}}{ 28.7 }\end{tabular}
% & \begin{tabular}[c]{@{}c@{}}{ \textbf{29.8} }\end{tabular}
% & \begin{tabular}[c]{@{}c@{}}{ 39.4 }\end{tabular}
% \\
% & \begin{tabular}[c]{@{}c@{}}\textrm{ Random }\end{tabular}
% & \begin{tabular}[c]{@{}c@{}}{ \textbf{50.6} }\end{tabular}
% & \begin{tabular}[c]{@{}c@{}}{ \textbf{59.9} }\end{tabular}
% & \begin{tabular}[c]{@{}c@{}}{ \textbf{23.8} }\end{tabular}
% & \begin{tabular}[c]{@{}c@{}}{ \textbf{24.1} }\end{tabular}
% & \begin{tabular}[c]{@{}c@{}}{ 32.4 }\end{tabular}
% & \begin{tabular}[c]{@{}c@{}}{ \textbf{45.4} }\end{tabular}
% & \begin{tabular}[c]{@{}c@{}}{ 15.0 }\end{tabular}
% & \begin{tabular}[c]{@{}c@{}}{ \textbf{30.7} }\end{tabular}
% & \begin{tabular}[c]{@{}c@{}}{ 26.7 }\end{tabular}
% & \begin{tabular}[c]{@{}c@{}}{ 39.5 }\end{tabular}
\\
\midrule
% # ER ###############################################################

% DER ++ ###############################################################
\multirow{2}{*}{DER++~\cite{buzzega2020dark}}                                                         
& \begin{tabular}[c]{@{}c@{}}\textrm{ -- }\end{tabular}
& \begin{tabular}[c]{@{}c@{}}{ {23.64}\,($\pm$0.32) }\end{tabular}
& \begin{tabular}[c]{@{}c@{}}{ {33.43}\,($\pm$0.73) }\end{tabular}
& \begin{tabular}[c]{@{}c@{}}{ {59.76}\,($\pm$0.76) }\end{tabular}
& \begin{tabular}[c]{@{}c@{}}{ {28.20}\,($\pm$1.48) }\end{tabular}
& \begin{tabular}[c]{@{}c@{}}{ {44.20}\,($\pm$1.01) }\end{tabular}
& \begin{tabular}[c]{@{}c@{}}{ {63.00}\,($\pm$4.62) }\end{tabular}
% & \begin{tabular}[c]{@{}c@{}}{ 12.3 }\end{tabular}
% & \begin{tabular}[c]{@{}c@{}}{ 28.2 }\end{tabular}
% & \begin{tabular}[c]{@{}c@{}}{ 22.7 }\end{tabular}
% & \begin{tabular}[c]{@{}c@{}}{ 37.9 }\end{tabular}
\\
& \begin{tabular}[c]{@{}c@{}}\textrm{ SDOCL }\end{tabular}
& \begin{tabular}[c]{@{}c@{}}{ \textbf{25.14}\,($\pm$0.27) }\end{tabular}
& \begin{tabular}[c]{@{}c@{}}{ \textbf{31.11}\,($\pm$1.15) }\end{tabular}
& \begin{tabular}[c]{@{}c@{}}{ \textbf{62.56}\,($\pm$0.73) }\end{tabular}
& \begin{tabular}[c]{@{}c@{}}{ \textbf{23.68}\,($\pm$0.98) }\end{tabular}
& \begin{tabular}[c]{@{}c@{}}{ \textbf{45.42}\,($\pm$0.54) }\end{tabular}
& \begin{tabular}[c]{@{}c@{}}{ \textbf{60.73}\,($\pm$5.06) }\end{tabular}
% & \begin{tabular}[c]{@{}c@{}}{ \textbf{13.8} }\end{tabular}
% & \begin{tabular}[c]{@{}c@{}}{ \textbf{29.5} }\end{tabular}
% & \begin{tabular}[c]{@{}c@{}}{ \textbf{23.5} }\end{tabular}
% & \begin{tabular}[c]{@{}c@{}}{ \textbf{38.9} }\end{tabular}
% \\
% & \begin{tabular}[c]{@{}c@{}}\textrm{ Random }\end{tabular}
% & \begin{tabular}[c]{@{}c@{}}{ \textbf{51.1} }\end{tabular}
% & \begin{tabular}[c]{@{}c@{}}{ \textbf{61.1} }\end{tabular}
% & \begin{tabular}[c]{@{}c@{}}{ \textbf{21.1} }\end{tabular}
% & \begin{tabular}[c]{@{}c@{}}{ 23.2 }\end{tabular}
% & \begin{tabular}[c]{@{}c@{}}{ \textbf{30.6 }}\end{tabular}
% & \begin{tabular}[c]{@{}c@{}}{ \textbf{43.5} }\end{tabular}
% & \begin{tabular}[c]{@{}c@{}}{ \textbf{19.6} }\end{tabular}
% & \begin{tabular}[c]{@{}c@{}}{ \textbf{29.0} }\end{tabular}
% & \begin{tabular}[c]{@{}c@{}}{ \textbf{26.7} }\end{tabular}
% & \begin{tabular}[c]{@{}c@{}}{ \textbf{38.5} }\end{tabular}
\\
\midrule
% % # ++ ###############################################################

% # MIR ################################################################
\multirow{2}{*}{MIR~\cite{mir}}                                               
& \begin{tabular}[c]{@{}c@{}}\textrm{ -- }\end{tabular}
& \begin{tabular}[c]{@{}c@{}}{ {20.75}\,($\pm$0.56) }\end{tabular}
& \begin{tabular}[c]{@{}c@{}}{ {25.32}\,($\pm$1.69) }\end{tabular}
& \begin{tabular}[c]{@{}c@{}}{ {51.54}\,($\pm$0.50) }\end{tabular}
& \begin{tabular}[c]{@{}c@{}}{ {58.42}\,($\pm$1.28) }\end{tabular}
& \begin{tabular}[c]{@{}c@{}}{ {39.34}\,($\pm$1.18) }\end{tabular}
& \begin{tabular}[c]{@{}c@{}}{ {41.07}\,($\pm$1.99) }\end{tabular}
% & \begin{tabular}[c]{@{}c@{}}{ 16.9 }\end{tabular}
% & \begin{tabular}[c]{@{}c@{}}{ 28.9 }\end{tabular}
% & \begin{tabular}[c]{@{}c@{}}{ 37.3 }\end{tabular}
% & \begin{tabular}[c]{@{}c@{}}{ 46.1 }\end{tabular}
\\
& \begin{tabular}[c]{@{}c@{}}\textrm{ SDOCL }\end{tabular}
& \begin{tabular}[c]{@{}c@{}}{ \textbf{22.44}\,($\pm$0.13) }\end{tabular}
& \begin{tabular}[c]{@{}c@{}}{ \textbf{24.83}\,($\pm$1.04) }\end{tabular}
& \begin{tabular}[c]{@{}c@{}}{ {51.63}\,($\pm$0.56) }\end{tabular}
& \begin{tabular}[c]{@{}c@{}}{ \textbf{56.25}\,($\pm$1.58) }\end{tabular}
& \begin{tabular}[c]{@{}c@{}}{ \textbf{42.01}\,($\pm$0.93) }\end{tabular}
& \begin{tabular}[c]{@{}c@{}}{ \textbf{39.25}\,($\pm$4.47) }\end{tabular}

% & \begin{tabular}[c]{@{}c@{}}{ \textbf{18.9} }\end{tabular}
% & \begin{tabular}[c]{@{}c@{}}{ \textbf{36.5} }\end{tabular}
% & \begin{tabular}[c]{@{}c@{}}{ \textbf{39.4}}\end{tabular}
% & \begin{tabular}[c]{@{}c@{}}{ \textbf{50.7} }\end{tabular}
% \\
% & \begin{tabular}[c]{@{}c@{}}\textrm{ Random }\end{tabular}
% & \begin{tabular}[c]{@{}c@{}}{ \textbf{62.7} }\end{tabular}
% & \begin{tabular}[c]{@{}c@{}}{ \textbf{69.5} }\end{tabular}
% & \begin{tabular}[c]{@{}c@{}}{ 35.0 }\end{tabular}
% & \begin{tabular}[c]{@{}c@{}}{ \textbf{31.1} }\end{tabular}
% & \begin{tabular}[c]{@{}c@{}}{ \textbf{52.4} }\end{tabular}
% & \begin{tabular}[c]{@{}c@{}}{ \textbf{56.5} }\end{tabular}
% & \begin{tabular}[c]{@{}c@{}}{ \textbf{20.0} }\end{tabular}
% & \begin{tabular}[c]{@{}c@{}}{ \textbf{33.6} }\end{tabular}
% & \begin{tabular}[c]{@{}c@{}}{\textbf{39.8} }\end{tabular}
% & \begin{tabular}[c]{@{}c@{}}{ \textbf{50.6} }\end{tabular}
\\
\midrule

% # GSS ################################################################
\multirow{2}{*}{GSS~\cite{aljundi2019gradient}}                                               
& \begin{tabular}[c]{@{}c@{}}\textrm{ -- }\end{tabular}
& \begin{tabular}[c]{@{}c@{}}{ {21.77}\,($\pm$0.34) }\end{tabular}
& \begin{tabular}[c]{@{}c@{}}{ {27.94}\,($\pm$0.80) }\end{tabular}
& \begin{tabular}[c]{@{}c@{}}{ {46.04}\,($\pm$0.42) }\end{tabular}
& \begin{tabular}[c]{@{}c@{}}{ {69.66}\,($\pm$0.71) }\end{tabular}
& \begin{tabular}[c]{@{}c@{}}{ {40.33}\,($\pm$0.63) }\end{tabular}
& \begin{tabular}[c]{@{}c@{}}{ {71.53}\,($\pm$2.01) }\end{tabular}

% & \begin{tabular}[c]{@{}c@{}}{ 16.9 }\end{tabular}
% & \begin{tabular}[c]{@{}c@{}}{ 28.9 }\end{tabular}
% & \begin{tabular}[c]{@{}c@{}}{ 37.3 }\end{tabular}
% & \begin{tabular}[c]{@{}c@{}}{ 46.1 }\end{tabular}
\\
& \begin{tabular}[c]{@{}c@{}}\textrm{ SDOCL }\end{tabular}
& \begin{tabular}[c]{@{}c@{}}{ \textbf{23.69}\,($\pm$0.16) }\end{tabular}
& \begin{tabular}[c]{@{}c@{}}{ \textbf{28.41}\,($\pm$1.00) }\end{tabular}
& \begin{tabular}[c]{@{}c@{}}{ \textbf{49.05}\,($\pm$0.46) }\end{tabular}
& \begin{tabular}[c]{@{}c@{}}{ \textbf{69.22}\,($\pm$1.53) }\end{tabular}
& \begin{tabular}[c]{@{}c@{}}{ \textbf{41.26}\,($\pm$0.57) }\end{tabular}
& \begin{tabular}[c]{@{}c@{}}{ \textbf{68.53}\,($\pm$1.87) }\end{tabular}

% & \begin{tabular}[c]{@{}c@{}}{ \textbf{18.9} }\end{tabular}
% & \begin{tabular}[c]{@{}c@{}}{ \textbf{36.5} }\end{tabular}
% & \begin{tabular}[c]{@{}c@{}}{ \textbf{39.4}}\end{tabular}
% & \begin{tabular}[c]{@{}c@{}}{ \textbf{50.7} }\end{tabular}
% \\
% & \begin{tabular}[c]{@{}c@{}}\textrm{ Random }\end{tabular}
% & \begin{tabular}[c]{@{}c@{}}{ \textbf{62.7} }\end{tabular}
% & \begin{tabular}[c]{@{}c@{}}{ \textbf{69.5} }\end{tabular}
% & \begin{tabular}[c]{@{}c@{}}{ 35.0 }\end{tabular}
% & \begin{tabular}[c]{@{}c@{}}{ \textbf{31.1} }\end{tabular}
% & \begin{tabular}[c]{@{}c@{}}{ \textbf{52.4} }\end{tabular}
% & \begin{tabular}[c]{@{}c@{}}{ \textbf{56.5} }\end{tabular}
% & \begin{tabular}[c]{@{}c@{}}{ \textbf{20.0} }\end{tabular}
% & \begin{tabular}[c]{@{}c@{}}{ \textbf{33.6} }\end{tabular}
% & \begin{tabular}[c]{@{}c@{}}{\textbf{39.8} }\end{tabular}
% & \begin{tabular}[c]{@{}c@{}}{ \textbf{50.6} }\end{tabular}
\\
\midrule

% # ASER ################################################################
\multirow{2}{*}{ASER~\cite{shim2021online}}                                               
& \begin{tabular}[c]{@{}c@{}}\textrm{ -- }\end{tabular}
& \begin{tabular}[c]{@{}c@{}}{ {32.68}\,($\pm$0.10) }\end{tabular}
& \begin{tabular}[c]{@{}c@{}}{ {41.77}\,($\pm$0.41) }\end{tabular}
& \begin{tabular}[c]{@{}c@{}}{ {50.32}\,($\pm$0.45) }\end{tabular}
& \begin{tabular}[c]{@{}c@{}}{ {57.77}\,($\pm$3.33) }\end{tabular}
& \begin{tabular}[c]{@{}c@{}}{ {39.70}\,($\pm$0.72) }\end{tabular}
& \begin{tabular}[c]{@{}c@{}}{ {62.63}\,($\pm$2.05) }\end{tabular}

% & \begin{tabular}[c]{@{}c@{}}{ 16.9 }\end{tabular}
% & \begin{tabular}[c]{@{}c@{}}{ 28.9 }\end{tabular}
% & \begin{tabular}[c]{@{}c@{}}{ 37.3 }\end{tabular}
% & \begin{tabular}[c]{@{}c@{}}{ 46.1 }\end{tabular}
\\
& \begin{tabular}[c]{@{}c@{}}\textrm{ SDOCL }\end{tabular}
& \begin{tabular}[c]{@{}c@{}}{ \textbf{33.43}\,($\pm$0.38) }\end{tabular}
& \begin{tabular}[c]{@{}c@{}}{ \textbf{39.54}\,($\pm$0.81) }\end{tabular}
& \begin{tabular}[c]{@{}c@{}}{ \textbf{51.32}\,($\pm$0.32) }\end{tabular}
& \begin{tabular}[c]{@{}c@{}}{ \textbf{57.54}\,($\pm$0.75) }\end{tabular}
& \begin{tabular}[c]{@{}c@{}}{ \textbf{41.60}\,($\pm$0.76) }\end{tabular}
& \begin{tabular}[c]{@{}c@{}}{ \textbf{57.50}\,($\pm$3.18) }\end{tabular}

% & \begin{tabular}[c]{@{}c@{}}{ \textbf{18.9} }\end{tabular}
% & \begin{tabular}[c]{@{}c@{}}{ \textbf{36.5} }\end{tabular}
% & \begin{tabular}[c]{@{}c@{}}{ \textbf{39.4}}\end{tabular}
% & \begin{tabular}[c]{@{}c@{}}{ \textbf{50.7} }\end{tabular}
% \\
% & \begin{tabular}[c]{@{}c@{}}\textrm{ Random }\end{tabular}
% & \begin{tabular}[c]{@{}c@{}}{ \textbf{62.7} }\end{tabular}
% & \begin{tabular}[c]{@{}c@{}}{ \textbf{69.5} }\end{tabular}
% & \begin{tabular}[c]{@{}c@{}}{ 35.0 }\end{tabular}
% & \begin{tabular}[c]{@{}c@{}}{ \textbf{31.1} }\end{tabular}
% & \begin{tabular}[c]{@{}c@{}}{ \textbf{52.4} }\end{tabular}
% & \begin{tabular}[c]{@{}c@{}}{ \textbf{56.5} }\end{tabular}
% & \begin{tabular}[c]{@{}c@{}}{ \textbf{20.0} }\end{tabular}
% & \begin{tabular}[c]{@{}c@{}}{ \textbf{33.6} }\end{tabular}
% & \begin{tabular}[c]{@{}c@{}}{\textbf{39.8} }\end{tabular}
% & \begin{tabular}[c]{@{}c@{}}{ \textbf{50.6} }\end{tabular}
\\
\bottomrule

\end{tabular}
}
\label{tbl:overall_comparison_biased_setup}
\end{table*}
