# Supplementary material for: Adaptive Shortcut Debiasing for Online Continual Learning
Source: arXiv:2312.08677 source file (2023-12-14)
Supplement: Supplementary file 5 [file performance_biased_setup_improv.tex]

\newcolumntype{C}[1]{>{\centering\arraybackslash}p{#1}}
% \bgroup
% make the row margin compact
\begin{table*}[t]
% \small
\scriptsize
% \small
% \label{tbl:RegionBuzComparison}
\centering
\caption{Average accuracy\,(the higher, the better) and forgetting\,(the lower, the better) on Split CIFAR-100, Split CIFAR-10, and Split ImageNet-9 for the biased setup. The highest values are marked in bold. }
% \vspace*{-0.3cm}
\resizebox{1.0\linewidth}{!}{%
\begin{tabular}[c]
% {@{}c|c|C{1.3cm}C{1.3cm}C{1.3cm}C{1.3cm}C{1.3cm}C{1.3cm}C{1.3cm}C{1.7cm}@{}}
{@{}l|c||C{1.85cm}c|C{1.85cm}c|C{1.85cm}cc@{}}
% {@{}c|c|ccccccccc@{}}
\toprule
\multicolumn{1}{c|}{} & \multicolumn{1}{c||}{} & \multicolumn{6}{c}{\textbf{\underline{    Biased Setup    }}} \\
% & \multicolumn{4}{c}{\textbf{{    Unbiased Setup   }}} \\
\multicolumn{1}{c|}{\textbf{OCL}} & \multicolumn{1}{c||}{\textbf{Debias}} & \multicolumn{2}{c}{\textbf{Split CIFAR-100}} & \multicolumn{2}{c}{\textbf{Split CIFAR-10}} & \multicolumn{2}{c}{\textbf{Split ImageNet-9}} \\
% & \multicolumn{2}{c}{\textbf{IN-OnlyFG}} & \multicolumn{2}{c}{\textbf{IN-Stylized}} \\
% \smallskip
\multicolumn{1}{c|}{\textbf{Method}}
& \multicolumn{1}{c||}{\textbf{Method}}
& \multicolumn{1}{c}{\bm{$A_{avg}$}\,($\uparrow$)}
& \multicolumn{1}{c|}{\bm{$F_{last}$}\,($\downarrow$)}
& \multicolumn{1}{c}{\bm{$A_{avg}$}\,($\uparrow$)}
& \multicolumn{1}{c|}{\bm{$F_{last}$}\,($\downarrow$)}
& \multicolumn{1}{c}{\bm{$A_{avg}$}\,($\uparrow$)}
& \multicolumn{1}{c}{\bm{$F_{last}$}\,($\downarrow$)}
% & \multicolumn{1}{c}{\bm{$A_{avg}$}}
% & \multicolumn{1}{c|}{\bm{$F_{last}$}}
% & \multicolumn{1}{c}{\bm{$A_{avg}$}}
% & \multicolumn{1}{c}{\bm{$F_{last}$}}
\\ \toprule
% # ER ###############################################################
\multirow{3}{*}{ER~\cite{rolnick2019experience}}                                
& \begin{tabular}[c]{@{}c@{}}\textrm{ -- }\end{tabular}
& \begin{tabular}[c]{@{}c@{}}{ {25.34}\,($\pm$0.18) }\end{tabular}
& \begin{tabular}[c]{@{}c@{}}{ {19.22}\,($\pm$0.25) }\end{tabular}
& \begin{tabular}[c]{@{}c@{}}{ {55.36}\,($\pm$0.30) }\end{tabular}
& \begin{tabular}[c]{@{}c@{}}{ {39.89}\,($\pm$2.35) }\end{tabular}
& \begin{tabular}[c]{@{}c@{}}{ {46.05}\,($\pm$0.20) }\end{tabular}
& \begin{tabular}[c]{@{}c@{}}{ {55.80}\,($\pm$1.82) }\end{tabular}
\\
& \begin{tabular}[c]{@{}c@{}}\textrm{ \algname{} }\end{tabular}
& \begin{tabular}[c]{@{}c@{}}{ \textbf{26.45}\,($\pm$0.17) }\end{tabular}
& \begin{tabular}[c]{@{}c@{}}{ \textbf{18.28}\,($\pm$1.31) }\end{tabular}
& \begin{tabular}[c]{@{}c@{}}{ \textbf{61.02}\,($\pm$0.61) }\end{tabular}
& \begin{tabular}[c]{@{}c@{}}{ \textbf{37.60}\,($\pm$1.89) }\end{tabular}
& \begin{tabular}[c]{@{}c@{}}{ \textbf{48.86}\,($\pm$0.43) }\end{tabular}
& \begin{tabular}[c]{@{}c@{}}{ \textbf{44.01}\,($\pm$3.76) }\end{tabular}
\\
\addlinespace[0.15ex]\cline{2-8}\addlinespace[0.6ex]
& \begin{tabular}[c]{@{}c@{}}\textrm{ {Rel. Improv.} }\end{tabular}
& \begin{tabular}[c]{@{}c@{}}{ 4.38\% }\end{tabular}
& \begin{tabular}[c]{@{}c@{}}{ 4.89\% }\end{tabular}
& \begin{tabular}[c]{@{}c@{}}{ 10.22\% }\end{tabular}
& \begin{tabular}[c]{@{}c@{}}{ 5.74\% }\end{tabular}
& \begin{tabular}[c]{@{}c@{}}{ 6.11\% }\end{tabular}
& \begin{tabular}[c]{@{}c@{}}{ 21.13\% }\end{tabular}
\\
\midrule
% # ER ###############################################################

% DER ++ ###############################################################
\multirow{3}{*}{DER++~\cite{buzzega2020dark}}                                                         
& \begin{tabular}[c]{@{}c@{}}\textrm{ -- }\end{tabular}
& \begin{tabular}[c]{@{}c@{}}{ {23.64}\,($\pm$0.32) }\end{tabular}
& \begin{tabular}[c]{@{}c@{}}{ {33.43}\,($\pm$0.73) }\end{tabular}
& \begin{tabular}[c]{@{}c@{}}{ {59.76}\,($\pm$0.76) }\end{tabular}
& \begin{tabular}[c]{@{}c@{}}{ {28.20}\,($\pm$1.48) }\end{tabular}
& \begin{tabular}[c]{@{}c@{}}{ {44.20}\,($\pm$1.01) }\end{tabular}
& \begin{tabular}[c]{@{}c@{}}{ {63.00}\,($\pm$4.62) }\end{tabular}
% & \begin{tabular}[c]{@{}c@{}}{ 12.3 }\end{tabular}
% & \begin{tabular}[c]{@{}c@{}}{ 28.2 }\end{tabular}
% & \begin{tabular}[c]{@{}c@{}}{ 22.7 }\end{tabular}
% & \begin{tabular}[c]{@{}c@{}}{ 37.9 }\end{tabular}
\\
& \begin{tabular}[c]{@{}c@{}}\textrm{ \algname{} }\end{tabular}
& \begin{tabular}[c]{@{}c@{}}{ \textbf{25.14}\,($\pm$0.27) }\end{tabular}
& \begin{tabular}[c]{@{}c@{}}{ \textbf{31.11}\,($\pm$1.15) }\end{tabular}
& \begin{tabular}[c]{@{}c@{}}{ \textbf{62.56}\,($\pm$0.73) }\end{tabular}
& \begin{tabular}[c]{@{}c@{}}{ \textbf{23.68}\,($\pm$0.98) }\end{tabular}
& \begin{tabular}[c]{@{}c@{}}{ \textbf{45.42}\,($\pm$0.54) }\end{tabular}
& \begin{tabular}[c]{@{}c@{}}{ \textbf{60.73}\,($\pm$5.06) }\end{tabular}
\\
\addlinespace[0.15ex]\cline{2-8}\addlinespace[0.6ex]
& \begin{tabular}[c]{@{}c@{}}\textrm{ {Rel. Improv}. }\end{tabular}
& \begin{tabular}[c]{@{}c@{}}{ 6.35\% }\end{tabular}
& \begin{tabular}[c]{@{}c@{}}{ 6.94\% }\end{tabular}
& \begin{tabular}[c]{@{}c@{}}{ 4.69\% }\end{tabular}
& \begin{tabular}[c]{@{}c@{}}{ 16.03\% }\end{tabular}
& \begin{tabular}[c]{@{}c@{}}{ 2.76\% }\end{tabular}
& \begin{tabular}[c]{@{}c@{}}{ 3.60\% }\end{tabular}
\\
\midrule
% % # ++ ###############################################################

% # MIR ################################################################
\multirow{3}{*}{MIR~\cite{mir}}                                               
& \begin{tabular}[c]{@{}c@{}}\textrm{ -- }\end{tabular}
& \begin{tabular}[c]{@{}c@{}}{ {20.75}\,($\pm$0.56) }\end{tabular}
& \begin{tabular}[c]{@{}c@{}}{ {25.32}\,($\pm$1.69) }\end{tabular}
& \begin{tabular}[c]{@{}c@{}}{ {51.54}\,($\pm$0.50) }\end{tabular}
& \begin{tabular}[c]{@{}c@{}}{ {58.42}\,($\pm$1.28) }\end{tabular}
& \begin{tabular}[c]{@{}c@{}}{ {39.34}\,($\pm$1.18) }\end{tabular}
& \begin{tabular}[c]{@{}c@{}}{ {41.07}\,($\pm$1.99) }\end{tabular}
% & \begin{tabular}[c]{@{}c@{}}{ 16.9 }\end{tabular}
% & \begin{tabular}[c]{@{}c@{}}{ 28.9 }\end{tabular}
% & \begin{tabular}[c]{@{}c@{}}{ 37.3 }\end{tabular}
% & \begin{tabular}[c]{@{}c@{}}{ 46.1 }\end{tabular}
\\
& \begin{tabular}[c]{@{}c@{}}\textrm{ \algname{} }\end{tabular}
& \begin{tabular}[c]{@{}c@{}}{ \textbf{22.44}\,($\pm$0.13) }\end{tabular}
& \begin{tabular}[c]{@{}c@{}}{ \textbf{24.83}\,($\pm$1.04) }\end{tabular}
& \begin{tabular}[c]{@{}c@{}}{ \textbf{51.63}\,($\pm$0.56) }\end{tabular}
& \begin{tabular}[c]{@{}c@{}}{ \textbf{56.25}\,($\pm$1.58) }\end{tabular}
& \begin{tabular}[c]{@{}c@{}}{ \textbf{42.01}\,($\pm$0.93) }\end{tabular}
& \begin{tabular}[c]{@{}c@{}}{ \textbf{39.25}\,($\pm$4.47) }\end{tabular}
\\
\addlinespace[0.15ex]\cline{2-8}\addlinespace[0.6ex]
& \begin{tabular}[c]{@{}c@{}}\textrm{ {Rel. Improv.} }\end{tabular}
& \begin{tabular}[c]{@{}c@{}}{ 8.14\% }\end{tabular}
& \begin{tabular}[c]{@{}c@{}}{ 1.94\% }\end{tabular}
& \begin{tabular}[c]{@{}c@{}}{ 0.17\% }\end{tabular}
& \begin{tabular}[c]{@{}c@{}}{ 3.71\% }\end{tabular}
& \begin{tabular}[c]{@{}c@{}}{ 6.79\% }\end{tabular}
& \begin{tabular}[c]{@{}c@{}}{ 4.43\% }\end{tabular}
\\
\midrule

% # GSS ################################################################
\multirow{3}{*}{GSS~\cite{aljundi2019gradient}}                                               
& \begin{tabular}[c]{@{}c@{}}\textrm{ -- }\end{tabular}
& \begin{tabular}[c]{@{}c@{}}{ {21.77}\,($\pm$0.34) }\end{tabular}
& \begin{tabular}[c]{@{}c@{}}{ \textbf{27.94}\,($\pm$0.80) }\end{tabular}
& \begin{tabular}[c]{@{}c@{}}{ {46.04}\,($\pm$0.42) }\end{tabular}
& \begin{tabular}[c]{@{}c@{}}{ {69.66}\,($\pm$0.71) }\end{tabular}
& \begin{tabular}[c]{@{}c@{}}{ {40.33}\,($\pm$0.63) }\end{tabular}
& \begin{tabular}[c]{@{}c@{}}{ {71.53}\,($\pm$2.01) }\end{tabular}
\\
& \begin{tabular}[c]{@{}c@{}}\textrm{ \algname{} }\end{tabular}
& \begin{tabular}[c]{@{}c@{}}{ \textbf{23.69}\,($\pm$0.16) }\end{tabular}
& \begin{tabular}[c]{@{}c@{}}{ {28.41}\,($\pm$1.00) }\end{tabular}
& \begin{tabular}[c]{@{}c@{}}{ \textbf{49.05}\,($\pm$0.46) }\end{tabular}
& \begin{tabular}[c]{@{}c@{}}{ \textbf{69.22}\,($\pm$1.53) }\end{tabular}
& \begin{tabular}[c]{@{}c@{}}{ \textbf{41.26}\,($\pm$0.57) }\end{tabular}
& \begin{tabular}[c]{@{}c@{}}{ \textbf{68.53}\,($\pm$1.87) }\end{tabular}
\\
\addlinespace[0.15ex]\cline{2-8}\addlinespace[0.6ex]
& \begin{tabular}[c]{@{}c@{}}\textrm{ {Rel. Improv.} }\end{tabular}
& \begin{tabular}[c]{@{}c@{}}{ 8.82\% }\end{tabular}
& \begin{tabular}[c]{@{}c@{}}{ -1.68\% }\end{tabular}
& \begin{tabular}[c]{@{}c@{}}{ 6.54\% }\end{tabular}
& \begin{tabular}[c]{@{}c@{}}{ 0.63\% }\end{tabular}
& \begin{tabular}[c]{@{}c@{}}{ 2.31\% }\end{tabular}
& \begin{tabular}[c]{@{}c@{}}{ 4.19\% }\end{tabular}
\\
\midrule

% # ASER ################################################################
\multirow{3}{*}{ASER~\cite{shim2021online}}                                               
& \begin{tabular}[c]{@{}c@{}}\textrm{ -- }\end{tabular}
& \begin{tabular}[c]{@{}c@{}}{ {32.68}\,($\pm$0.10) }\end{tabular}
& \begin{tabular}[c]{@{}c@{}}{ {41.77}\,($\pm$0.41) }\end{tabular}
& \begin{tabular}[c]{@{}c@{}}{ {50.32}\,($\pm$0.45) }\end{tabular}
& \begin{tabular}[c]{@{}c@{}}{ {57.77}\,($\pm$3.33) }\end{tabular}
& \begin{tabular}[c]{@{}c@{}}{ {39.70}\,($\pm$0.72) }\end{tabular}
& \begin{tabular}[c]{@{}c@{}}{ {62.63}\,($\pm$2.05) }\end{tabular}

% & \begin{tabular}[c]{@{}c@{}}{ 16.9 }\end{tabular}
% & \begin{tabular}[c]{@{}c@{}}{ 28.9 }\end{tabular}
% & \begin{tabular}[c]{@{}c@{}}{ 37.3 }\end{tabular}
% & \begin{tabular}[c]{@{}c@{}}{ 46.1 }\end{tabular}
\\
& \begin{tabular}[c]{@{}c@{}}\textrm{ \algname{} }\end{tabular}
& \begin{tabular}[c]{@{}c@{}}{ \textbf{33.43}\,($\pm$0.38) }\end{tabular}
& \begin{tabular}[c]{@{}c@{}}{ \textbf{39.54}\,($\pm$0.81) }\end{tabular}
& \begin{tabular}[c]{@{}c@{}}{ \textbf{51.32}\,($\pm$0.32) }\end{tabular}
& \begin{tabular}[c]{@{}c@{}}{ \textbf{57.54}\,($\pm$0.75) }\end{tabular}
& \begin{tabular}[c]{@{}c@{}}{ \textbf{41.60}\,($\pm$0.76) }\end{tabular}
& \begin{tabular}[c]{@{}c@{}}{ \textbf{57.50}\,($\pm$3.18) }\end{tabular}
\\
\addlinespace[0.15ex]\cline{2-8}\addlinespace[0.6ex]
& \begin{tabular}[c]{@{}c@{}}\textrm{ {Rel. Improv.} }\end{tabular}
& \begin{tabular}[c]{@{}c@{}}{ 2.29\% }\end{tabular}
& \begin{tabular}[c]{@{}c@{}}{ 5.34\% }\end{tabular}
& \begin{tabular}[c]{@{}c@{}}{ 1.99\% }\end{tabular}
& \begin{tabular}[c]{@{}c@{}}{ 0.40\% }\end{tabular}
& \begin{tabular}[c]{@{}c@{}}{ 4.79\% }\end{tabular}
& \begin{tabular}[c]{@{}c@{}}{ 8.19\% }\end{tabular}
\\
\bottomrule

\end{tabular}
}
\label{tbl:overall_comparison_biased_setup}
\vspace*{-0.2cm}
\end{table*}
