# Supplementary material for: Adaptive Shortcut Debiasing for Online Continual Learning
Source: arXiv:2312.08677 source file (2023-12-14)
Supplement: Supplementary file 6 [file performance_biased_unbiased_setup.tex]

\newcolumntype{C}[1]{>{\centering\arraybackslash}p{#1}}
% \bgroup
% make the row margin compact
\begin{table*}[t]
\small
% \scriptsize
% \small
% \label{tbl:RegionBuzComparison}
\centering
\caption{Average accuracy\,(higher is better) and forgetting\,(lower is better) on Split CIFAR-100, Split CIFAR-10, and Split ImageNet-9 for biased setup and Split ImageNet(IN)-\{OnlyFG, Stylized\} for unbiased setup. The mean of \emph{five} repetitions with different random initialization were reported. }
\resizebox{1.0\linewidth}{!}{%
\begin{tabular}[c]
% {@{}c|c|C{1.3cm}C{1.3cm}C{1.3cm}C{1.3cm}C{1.3cm}C{1.3cm}C{1.3cm}C{1.7cm}@{}}
% {@{}c|c||C{1.85cm}c|C{1.85cm}c|C{1.85cm}cc@{}}
{@{}l|ccccccccccc@{}}
\toprule
\multicolumn{1}{c|}{} & \multicolumn{6}{c|}{\textbf{\underline{    Biased Setup    }}} 
& \multicolumn{4}{c}{\textbf{\underline{    Unbiased Setup   }}} \\
% \multicolumn{1}{c|}{\textbf{OCL}} & \multicolumn{1}{c||}{\textbf{Debiasing}} 
\multicolumn{1}{c|}{\textbf{}}& \multicolumn{2}{c}{\textbf{Split CIFAR-100}} & \multicolumn{2}{c}{\textbf{Split CIFAR-10}} & \multicolumn{2}{c|}{\textbf{Split ImageNet-9}}
& \multicolumn{2}{c}{\textbf{Split IN-OnlyFG}} & \multicolumn{2}{c}{\textbf{Split IN-Stylized}} \\
% \smallskip
\multicolumn{1}{c|}{\textbf{Method}}
% & \multicolumn{1}{c||}{\textbf{Method}}
& \multicolumn{1}{c}{\bm{$A_{avg}$}\,($\uparrow$)}
& \multicolumn{1}{c|}{\bm{$F_{last}$}\,($\downarrow$)}
& \multicolumn{1}{c}{\bm{$A_{avg}$}\,($\uparrow$)}
& \multicolumn{1}{c|}{\bm{$F_{last}$}\,($\downarrow$)}
& \multicolumn{1}{c}{\bm{$A_{avg}$}\,($\uparrow$)}
& \multicolumn{1}{c|}{\bm{$F_{last}$}\,($\downarrow$)}
& \multicolumn{1}{c}{\bm{$A_{avg}$}\,($\uparrow$)}
& \multicolumn{1}{c|}{\bm{$F_{last}$}\,($\downarrow$)}
& \multicolumn{1}{c}{\bm{$A_{avg}$}\,($\uparrow$)}
& \multicolumn{1}{c}{\bm{$F_{last}$}\,($\downarrow$)}
\\ \toprule
% # ER ###############################################################
\multirow{1}{*}{ER~\cite{rolnick2019experience}}                                
% & \begin{tabular}[c]{@{}c@{}}\textrm{ -- }\end{tabular}
& \begin{tabular}[c]{@{}c@{}}{ {25.3}\,($\pm$0.2) }\end{tabular}
& \begin{tabular}[c]{@{}c@{}}{ {19.2}\,($\pm$0.3) }\end{tabular}
& \begin{tabular}[c]{@{}c@{}}{ {55.4}\,($\pm$0.3) }\end{tabular}
& \begin{tabular}[c]{@{}c@{}}{ {39.9}\,($\pm$2.4) }\end{tabular}
& \begin{tabular}[c]{@{}c@{}}{ {46.1}\,($\pm$0.2) }\end{tabular}
& \begin{tabular}[c]{@{}c@{}}{ {55.8}\,($\pm$1.8) }\end{tabular}
& \begin{tabular}[c]{@{}c@{}}{ {32.8}\,($\pm$0.4) }\end{tabular}
& \begin{tabular}[c]{@{}c@{}}{ {45.0}\,($\pm$1.5) }\end{tabular}
& \begin{tabular}[c]{@{}c@{}}{ {39.3}\,($\pm$0.3) }\end{tabular}
& \begin{tabular}[c]{@{}c@{}}{ {49.7}\,($\pm$0.9) }\end{tabular}

% & \begin{tabular}[c]{@{}c@{}}{ 17.6 }\end{tabular}
% & \begin{tabular}[c]{@{}c@{}}{ 28.9 }\end{tabular}
% & \begin{tabular}[c]{@{}c@{}}{ 29.1 }\end{tabular}
% & \begin{tabular}[c]{@{}c@{}}{ \textbf{40.3} }\end{tabular}
\\
\multirow{1}{*}{\textbf{~~$+$SDOCL}}  
% & \begin{tabular}[c]{@{}c@{}}\textrm{ SDOCL }\end{tabular}
& \begin{tabular}[c]{@{}c@{}}{ {26.5}\,($\pm$0.2) }\end{tabular}
& \begin{tabular}[c]{@{}c@{}}{ {18.3}\,($\pm$1.3) }\end{tabular}
& \begin{tabular}[c]{@{}c@{}}{ {61.0}\,($\pm$0.6) }\end{tabular}
& \begin{tabular}[c]{@{}c@{}}{ {37.6}\,($\pm$1.9) }\end{tabular}
& \begin{tabular}[c]{@{}c@{}}{ {48.9}\,($\pm$0.4) }\end{tabular}
& \begin{tabular}[c]{@{}c@{}}{ {44.0}\,($\pm$3.8) }\end{tabular}
& \begin{tabular}[c]{@{}c@{}}{ {35.9}\,($\pm$0.9) }\end{tabular}
& \begin{tabular}[c]{@{}c@{}}{ {47.8}\,($\pm$3.7) }\end{tabular}
& \begin{tabular}[c]{@{}c@{}}{ {41.3}\,($\pm$0.1) }\end{tabular}
& \begin{tabular}[c]{@{}c@{}}{ {38.9}\,($\pm$2.6) }\end{tabular}
% & \begin{tabular}[c]{@{}c@{}}{ \textbf{19.2} ($\pm$ 0.12) }\end{tabular}
% & \begin{tabular}[c]{@{}c@{}}{ 28.7 }\end{tabular}
% & \begin{tabular}[c]{@{}c@{}}{ \textbf{29.8} }\end{tabular}
% & \begin{tabular}[c]{@{}c@{}}{ 39.4 }\end{tabular}
% \\
% & \begin{tabular}[c]{@{}c@{}}\textrm{ Random }\end{tabular}
% & \begin{tabular}[c]{@{}c@{}}{ \textbf{50.6} }\end{tabular}
% & \begin{tabular}[c]{@{}c@{}}{ \textbf{59.9} }\end{tabular}
% & \begin{tabular}[c]{@{}c@{}}{ \textbf{23.8} }\end{tabular}
% & \begin{tabular}[c]{@{}c@{}}{ \textbf{24.1} }\end{tabular}
% & \begin{tabular}[c]{@{}c@{}}{ 32.4 }\end{tabular}
% & \begin{tabular}[c]{@{}c@{}}{ \textbf{45.4} }\end{tabular}
% & \begin{tabular}[c]{@{}c@{}}{ 15.0 }\end{tabular}
% & \begin{tabular}[c]{@{}c@{}}{ \textbf{30.7} }\end{tabular}
% & \begin{tabular}[c]{@{}c@{}}{ 26.7 }\end{tabular}
% & \begin{tabular}[c]{@{}c@{}}{ 39.5 }\end{tabular}
\\
\midrule
% # ER ###############################################################

% DER ++ ###############################################################
\multirow{1}{*}{DER++~\cite{buzzega2020dark}}                                                         
% & \begin{tabular}[c]{@{}c@{}}\textrm{ -- }\end{tabular}
& \begin{tabular}[c]{@{}c@{}}{ {23.6}\,($\pm$0.3) }\end{tabular}
& \begin{tabular}[c]{@{}c@{}}{ {33.4}\,($\pm$0.7) }\end{tabular}
& \begin{tabular}[c]{@{}c@{}}{ {59.8}\,($\pm$0.8) }\end{tabular}
& \begin{tabular}[c]{@{}c@{}}{ {28.2}\,($\pm$1.5) }\end{tabular}
& \begin{tabular}[c]{@{}c@{}}{ {44.2}\,($\pm$1.0) }\end{tabular}
& \begin{tabular}[c]{@{}c@{}}{ {63.0}\,($\pm$4.6) }\end{tabular}
& \begin{tabular}[c]{@{}c@{}}{ {33.2}\,($\pm$0.5) }\end{tabular}
& \begin{tabular}[c]{@{}c@{}}{ {61.6}\,($\pm$2.1) }\end{tabular}
& \begin{tabular}[c]{@{}c@{}}{ {37.8}\,($\pm$0.7) }\end{tabular}
& \begin{tabular}[c]{@{}c@{}}{ {60.3}\,($\pm$3.2) }\end{tabular}
% & \begin{tabular}[c]{@{}c@{}}{ 12.3 }\end{tabular}
% & \begin{tabular}[c]{@{}c@{}}{ 28.2 }\end{tabular}
% & \begin{tabular}[c]{@{}c@{}}{ 22.7 }\end{tabular}
% & \begin{tabular}[c]{@{}c@{}}{ 37.9 }\end{tabular}
\\
\multirow{1}{*}{\textbf{~~$+$SDOCL}}   
% & \begin{tabular}[c]{@{}c@{}}\textrm{ SDOCL }\end{tabular}
& \begin{tabular}[c]{@{}c@{}}{ {25.1}\,($\pm$0.3) }\end{tabular}
& \begin{tabular}[c]{@{}c@{}}{ {31.1}\,($\pm$1.2) }\end{tabular}
& \begin{tabular}[c]{@{}c@{}}{ {62.6}\,($\pm$0.7) }\end{tabular}
& \begin{tabular}[c]{@{}c@{}}{ {23.7}\,($\pm$1.0) }\end{tabular}
& \begin{tabular}[c]{@{}c@{}}{ {45.4}\,($\pm$0.5) }\end{tabular}
& \begin{tabular}[c]{@{}c@{}}{ {60.7}\,($\pm$5.1) }\end{tabular}
& \begin{tabular}[c]{@{}c@{}}{ {34.5}\,($\pm$0.7) }\end{tabular}
& \begin{tabular}[c]{@{}c@{}}{ {54.9}\,($\pm$3.2) }\end{tabular}
& \begin{tabular}[c]{@{}c@{}}{ {39.7}\,($\pm$0.4) }\end{tabular}
& \begin{tabular}[c]{@{}c@{}}{ {58.9}\,($\pm$4.1) }\end{tabular}
% & \begin{tabular}[c]{@{}c@{}}{ \textbf{13.8} }\end{tabular}
% & \begin{tabular}[c]{@{}c@{}}{ \textbf{29.5} }\end{tabular}
% & \begin{tabular}[c]{@{}c@{}}{ \textbf{23.5} }\end{tabular}
% & \begin{tabular}[c]{@{}c@{}}{ \textbf{38.9} }\end{tabular}
% \\
% & \begin{tabular}[c]{@{}c@{}}\textrm{ Random }\end{tabular}
% & \begin{tabular}[c]{@{}c@{}}{ \textbf{51.1} }\end{tabular}
% & \begin{tabular}[c]{@{}c@{}}{ \textbf{61.1} }\end{tabular}
% & \begin{tabular}[c]{@{}c@{}}{ \textbf{21.1} }\end{tabular}
% & \begin{tabular}[c]{@{}c@{}}{ 23.2 }\end{tabular}
% & \begin{tabular}[c]{@{}c@{}}{ \textbf{30.6 }}\end{tabular}
% & \begin{tabular}[c]{@{}c@{}}{ \textbf{43.5} }\end{tabular}
% & \begin{tabular}[c]{@{}c@{}}{ \textbf{19.6} }\end{tabular}
% & \begin{tabular}[c]{@{}c@{}}{ \textbf{29.0} }\end{tabular}
% & \begin{tabular}[c]{@{}c@{}}{ \textbf{26.7} }\end{tabular}
% & \begin{tabular}[c]{@{}c@{}}{ \textbf{38.5} }\end{tabular}
\\
\midrule
% % # ++ ###############################################################

% # MIR ################################################################
\multirow{1}{*}{MIR~\cite{mir}}                              

% & \begin{tabular}[c]{@{}c@{}}\textrm{ -- }\end{tabular}
& \begin{tabular}[c]{@{}c@{}}{ {20.8}\,($\pm$0.6) }\end{tabular}
& \begin{tabular}[c]{@{}c@{}}{ {25.3}\,($\pm$1.7) }\end{tabular}
& \begin{tabular}[c]{@{}c@{}}{ {51.5}\,($\pm$0.5) }\end{tabular}
& \begin{tabular}[c]{@{}c@{}}{ {58.4}\,($\pm$1.3) }\end{tabular}
& \begin{tabular}[c]{@{}c@{}}{ {39.3}\,($\pm$1.2) }\end{tabular}
& \begin{tabular}[c]{@{}c@{}}{ {41.1}\,($\pm$2.0) }\end{tabular}
& \begin{tabular}[c]{@{}c@{}}{ {32.1}\,($\pm$0.4) }\end{tabular}
& \begin{tabular}[c]{@{}c@{}}{ {38.9}\,($\pm$3.1) }\end{tabular}
& \begin{tabular}[c]{@{}c@{}}{ {34.0}\,($\pm$1.0) }\end{tabular}
& \begin{tabular}[c]{@{}c@{}}{ {40.7}\,($\pm$1.6) }\end{tabular}
% & \begin{tabular}[c]{@{}c@{}}{ 16.9 }\end{tabular}
% & \begin{tabular}[c]{@{}c@{}}{ 28.9 }\end{tabular}
% & \begin{tabular}[c]{@{}c@{}}{ 37.3 }\end{tabular}
% & \begin{tabular}[c]{@{}c@{}}{ 46.1 }\end{tabular}
\\
\multirow{1}{*}{\textbf{~~$+$SDOCL}}
% & \begin{tabular}[c]{@{}c@{}}\textrm{ SDOCL }\end{tabular}
& \begin{tabular}[c]{@{}c@{}}{ {22.4}\,($\pm$0.1) }\end{tabular}
& \begin{tabular}[c]{@{}c@{}}{ {24.8}\,($\pm$1.0) }\end{tabular}
& \begin{tabular}[c]{@{}c@{}}{ {51.6}\,($\pm$0.6) }\end{tabular}
& \begin{tabular}[c]{@{}c@{}}{ {56.3}\,($\pm$1.6) }\end{tabular}
& \begin{tabular}[c]{@{}c@{}}{ {42.0}\,($\pm$0.9) }\end{tabular}
& \begin{tabular}[c]{@{}c@{}}{ {39.3}\,($\pm$4.5) }\end{tabular}
& \begin{tabular}[c]{@{}c@{}}{ {35.4}\,($\pm$1.4) }\end{tabular}
& \begin{tabular}[c]{@{}c@{}}{ {36.0}\,($\pm$3.1) }\end{tabular}
& \begin{tabular}[c]{@{}c@{}}{ {36.1}\,($\pm$0.6) }\end{tabular}
& \begin{tabular}[c]{@{}c@{}}{ {38.3}\,($\pm$3.4) }\end{tabular}

% & \begin{tabular}[c]{@{}c@{}}{ \textbf{18.9} }\end{tabular}
% & \begin{tabular}[c]{@{}c@{}}{ \textbf{36.5} }\end{tabular}
% & \begin{tabular}[c]{@{}c@{}}{ \textbf{39.4}}\end{tabular}
% & \begin{tabular}[c]{@{}c@{}}{ \textbf{50.7} }\end{tabular}
% \\
% & \begin{tabular}[c]{@{}c@{}}\textrm{ Random }\end{tabular}
% & \begin{tabular}[c]{@{}c@{}}{ \textbf{62.7} }\end{tabular}
% & \begin{tabular}[c]{@{}c@{}}{ \textbf{69.5} }\end{tabular}
% & \begin{tabular}[c]{@{}c@{}}{ 35.0 }\end{tabular}
% & \begin{tabular}[c]{@{}c@{}}{ \textbf{31.1} }\end{tabular}
% & \begin{tabular}[c]{@{}c@{}}{ \textbf{52.4} }\end{tabular}
% & \begin{tabular}[c]{@{}c@{}}{ \textbf{56.5} }\end{tabular}
% & \begin{tabular}[c]{@{}c@{}}{ \textbf{20.0} }\end{tabular}
% & \begin{tabular}[c]{@{}c@{}}{ \textbf{33.6} }\end{tabular}
% & \begin{tabular}[c]{@{}c@{}}{\textbf{39.8} }\end{tabular}
% & \begin{tabular}[c]{@{}c@{}}{ \textbf{50.6} }\end{tabular}
\\
\midrule

% # GSS ################################################################
\multirow{1}{*}{GSS~\cite{aljundi2019gradient}}                                               
% & \begin{tabular}[c]{@{}c@{}}\textrm{ -- }\end{tabular}
& \begin{tabular}[c]{@{}c@{}}{ {21.8}\,($\pm$0.3) }\end{tabular}
& \begin{tabular}[c]{@{}c@{}}{ {27.9}\,($\pm$0.8) }\end{tabular}
& \begin{tabular}[c]{@{}c@{}}{ {46.0}\,($\pm$0.4) }\end{tabular}
& \begin{tabular}[c]{@{}c@{}}{ {69.7}\,($\pm$0.7) }\end{tabular}
& \begin{tabular}[c]{@{}c@{}}{ {40.3}\,($\pm$0.6) }\end{tabular}
& \begin{tabular}[c]{@{}c@{}}{ {71.5}\,($\pm$2.0) }\end{tabular}
& \begin{tabular}[c]{@{}c@{}}{ {34.5}\,($\pm$0.9) }\end{tabular}
& \begin{tabular}[c]{@{}c@{}}{ {65.6}\,($\pm$0.7) }\end{tabular}
& \begin{tabular}[c]{@{}c@{}}{ {35.3}\,($\pm$0.7) }\end{tabular}
& \begin{tabular}[c]{@{}c@{}}{ {64.2}\,($\pm$1.9) }\end{tabular}

% & \begin{tabular}[c]{@{}c@{}}{ 16.9 }\end{tabular}
% & \begin{tabular}[c]{@{}c@{}}{ 28.9 }\end{tabular}
% & \begin{tabular}[c]{@{}c@{}}{ 37.3 }\end{tabular}
% & \begin{tabular}[c]{@{}c@{}}{ 46.1 }\end{tabular}
\\
\multirow{1}{*}{\textbf{~~$+$SDOCL}}
% & \begin{tabular}[c]{@{}c@{}}\textrm{ SDOCL }\end{tabular}
& \begin{tabular}[c]{@{}c@{}}{ {23.7}\,($\pm$0.2) }\end{tabular}
& \begin{tabular}[c]{@{}c@{}}{ {28.4}\,($\pm$1.0) }\end{tabular}
& \begin{tabular}[c]{@{}c@{}}{ {49.1}\,($\pm$0.5) }\end{tabular}
& \begin{tabular}[c]{@{}c@{}}{ {69.2}\,($\pm$1.5) }\end{tabular}
& \begin{tabular}[c]{@{}c@{}}{ {41.3}\,($\pm$0.6) }\end{tabular}
& \begin{tabular}[c]{@{}c@{}}{ {68.5}\,($\pm$1.9) }\end{tabular}
& \begin{tabular}[c]{@{}c@{}}{ {36.5}\,($\pm$0.7) }\end{tabular}
& \begin{tabular}[c]{@{}c@{}}{ {61.6}\,($\pm$1.8) }\end{tabular}
& \begin{tabular}[c]{@{}c@{}}{ {35.9}\,($\pm$0.4) }\end{tabular}
& \begin{tabular}[c]{@{}c@{}}{ {62.3}\,($\pm$2.3) }\end{tabular}

% & \begin{tabular}[c]{@{}c@{}}{ \textbf{18.9} }\end{tabular}
% & \begin{tabular}[c]{@{}c@{}}{ \textbf{36.5} }\end{tabular}
% & \begin{tabular}[c]{@{}c@{}}{ \textbf{39.4}}\end{tabular}
% & \begin{tabular}[c]{@{}c@{}}{ \textbf{50.7} }\end{tabular}
% \\
% & \begin{tabular}[c]{@{}c@{}}\textrm{ Random }\end{tabular}
% & \begin{tabular}[c]{@{}c@{}}{ \textbf{62.7} }\end{tabular}
% & \begin{tabular}[c]{@{}c@{}}{ \textbf{69.5} }\end{tabular}
% & \begin{tabular}[c]{@{}c@{}}{ 35.0 }\end{tabular}
% & \begin{tabular}[c]{@{}c@{}}{ \textbf{31.1} }\end{tabular}
% & \begin{tabular}[c]{@{}c@{}}{ \textbf{52.4} }\end{tabular}
% & \begin{tabular}[c]{@{}c@{}}{ \textbf{56.5} }\end{tabular}
% & \begin{tabular}[c]{@{}c@{}}{ \textbf{20.0} }\end{tabular}
% & \begin{tabular}[c]{@{}c@{}}{ \textbf{33.6} }\end{tabular}
% & \begin{tabular}[c]{@{}c@{}}{\textbf{39.8} }\end{tabular}
% & \begin{tabular}[c]{@{}c@{}}{ \textbf{50.6} }\end{tabular}
\\
\midrule

% # ASER ################################################################
\multirow{1}{*}{ASER~\cite{shim2021online}}                                               
% & \begin{tabular}[c]{@{}c@{}}\textrm{ -- }\end{tabular}
& \begin{tabular}[c]{@{}c@{}}{ {32.7}\,($\pm$0.1) }\end{tabular}
& \begin{tabular}[c]{@{}c@{}}{ {41.8}\,($\pm$0.4) }\end{tabular}
& \begin{tabular}[c]{@{}c@{}}{ {50.3}\,($\pm$0.5) }\end{tabular}
& \begin{tabular}[c]{@{}c@{}}{ {57.8}\,($\pm$3.3) }\end{tabular}
& \begin{tabular}[c]{@{}c@{}}{ {39.7}\,($\pm$0.7) }\end{tabular}
& \begin{tabular}[c]{@{}c@{}}{ {62.6}\,($\pm$2.1) }\end{tabular}
& \begin{tabular}[c]{@{}c@{}}{ {30.2}\,($\pm$0.2) }\end{tabular}
& \begin{tabular}[c]{@{}c@{}}{ {60.2}\,($\pm$0.9) }\end{tabular}
& \begin{tabular}[c]{@{}c@{}}{ {33.6}\,($\pm$0.5) }\end{tabular}
& \begin{tabular}[c]{@{}c@{}}{ {56.8}\,($\pm$1.1) }\end{tabular}

% & \begin{tabular}[c]{@{}c@{}}{ 16.9 }\end{tabular}
% & \begin{tabular}[c]{@{}c@{}}{ 28.9 }\end{tabular}
% & \begin{tabular}[c]{@{}c@{}}{ 37.3 }\end{tabular}
% & \begin{tabular}[c]{@{}c@{}}{ 46.1 }\end{tabular}
\\
\multirow{1}{*}{\textbf{~~$+$SDOCL}}
% & \begin{tabular}[c]{@{}c@{}}\textrm{ SDOCL }\end{tabular}
& \begin{tabular}[c]{@{}c@{}}{ {33.4}\,($\pm$0.4) }\end{tabular}
& \begin{tabular}[c]{@{}c@{}}{ {39.5}\,($\pm$0.8) }\end{tabular}
& \begin{tabular}[c]{@{}c@{}}{ {51.3}\,($\pm$0.3) }\end{tabular}
& \begin{tabular}[c]{@{}c@{}}{ {57.5}\,($\pm$0.8) }\end{tabular}
& \begin{tabular}[c]{@{}c@{}}{ {41.6}\,($\pm$0.8) }\end{tabular}
& \begin{tabular}[c]{@{}c@{}}{ {57.5}\,($\pm$3.2) }\end{tabular}
& \begin{tabular}[c]{@{}c@{}}{ {31.2}\,($\pm$0.2) }\end{tabular}
& \begin{tabular}[c]{@{}c@{}}{ {49.6}\,($\pm$2.8) }\end{tabular}
& \begin{tabular}[c]{@{}c@{}}{ {35.5}\,($\pm$0.4) }\end{tabular}
& \begin{tabular}[c]{@{}c@{}}{ {52.6}\,($\pm$2.5) }\end{tabular}

\\
\bottomrule

\end{tabular}
}
\label{tbl:overall_comparison_biased_unbiased_setup}
\vspace{-1em}
\end{table*}
